# Supplementary material for: Towards Unconstrained 2D Pose Estimation of the Human Spine
Source: arXiv:2504.08110 source file (2025-04-10)
Supplement: Supplementary file 1 [file X_suppl.tex]

\clearpage
\setcounter{page}{1}
\maketitlesupplementary

\section{Additional Results}

\begin{figure}[ht]
    \includegraphics[clip,trim={0 2cm 0 0.5cm},width=0.195\columnwidth]{figures/teaser/0.png}
    \includegraphics[clip,trim={0 2cm 0 0.5cm},width=0.195\columnwidth]{figures/teaser/1.png}
    \includegraphics[clip,trim={0 2cm 0 0.5cm},width=0.195\columnwidth]{figures/teaser/2.png}
    \includegraphics[clip,trim={0 2cm 0 0.5cm},width=0.195\columnwidth]{figures/teaser/3.png}
    \includegraphics[clip,trim={0 2cm 0 0.5cm},width=0.195\columnwidth]{figures/teaser/4.png}
\end{figure}
